# Supplementary material for: A statistical approach to latent dynamic modeling with differential equations
Source: arXiv:2311.16286 ancillary file (2025-07-09)
Supplement: Supplementary file 1 [file Supplement.pdf]

# Supplementary Material for “A statistical approach to latent dynamic modeling with differential equations”

Maren Hackenberg, Astrid Pechmann, Clemens Kreutz,  
Janbernd Kirschner and Harald Binder

July 3, 2025

## Contents

|   |                                                                |   |
|---|----------------------------------------------------------------|---|
| 1 | Derivation of the analytical solution to the linear ODE system | 2 |
| 2 | Implementation details                                         | 3 |
| 3 | Sensitivity analysis                                           | 4 |
| 4 | Simulation design with a simpler ODE system                    | 5 |

# 1 Derivation of the analytical solution to the linear ODE system

In the following, we show how to arrive at the analytical solution in Equation 2 in the main text to the initial value problem from Equation 1 in the main text. For  $A \in \mathbb{R}^{d \times d}$ ,  $A \neq 0$  and  $c \in \mathbb{R}^d$ , we have

$$\begin{aligned} z'(t) &= A \cdot z(t) + c; \\ z(t_0) &= z_0. \end{aligned}$$

Subtracting  $A \cdot z(t)$  and multiplying by  $\exp(-At)$  yields

$$(z'(t) - Az(t)) \exp(-At) = c \cdot \exp(-At). \quad (1)$$

According to the product rule,

$$\frac{d}{dt}(z(t) \exp(-At)) = z'(t) \exp(-At) - Az(t) \exp(-At) = (z'(t) - Az(t)) \exp(-At),$$

and hence, substituting this identity in Equation (1) we obtain

$$\frac{d}{dt}(z(t) \exp(-At)) = c \exp(-At).$$

Integrating both sides yields

$$\begin{aligned} z(t) \exp(-At) &= \int_{t_0}^t c \exp(-As) ds + K \quad (\text{for some constant } K \in \mathbb{R}^d) \\ &= -A^{-1}c \exp(-At) + A^{-1}c \exp(-At_0) + K, \end{aligned}$$

and thus

$$\begin{aligned} z(t) &= (-A^{-1}c \exp(-At) + A^{-1}c \exp(-At_0) + K) \exp(At) \\ &= (A^{-1}c \exp(-At_0) + K) \exp(At) - A^{-1}c. \end{aligned} \quad (2)$$

Evaluating Equation (2) at  $t = t_0$ , we obtain

$$\begin{aligned} z(t_0) &= (A^{-1}c \exp(-At_0) + K) \exp(At_0) - A^{-1}c \\ &= A^{-1}c + K \exp(At_0) - A^{-1}c \\ &= K \exp(At_0), \end{aligned}$$

and thus  $K = z(t_0) \exp(-At_0) = z_0 \exp(-At_0)$ . Inserting this into Equation (2), we finally arrive at the analytical solution from Equation 2 in the main text:

$$\begin{aligned} z(t) &= (A^{-1}c \exp(-At_0) + z_0 \exp(-At_0)) \exp(At) - A^{-1}c \\ &= (A^{-1}c + z_0) \exp(A(t - t_0)) - A^{-1}c. \end{aligned}$$

## 2 Implementation details

We use differentiable programming for simultaneous optimization of the dynamic model and the VAE encoder and decoder. Differentiable programming (Innes 2019) is a new paradigm for flexibly coupling optimization of diverse model components. For an overview, see our own work Hackenberg et al. (2022a). Briefly, differentiable programming facilitates a combination of different modeling components, such as neural network and differential equations, by allowing for joint optimization of an overall loss function using automatic differentiation (Baydin et al. 2017). Thus, gradients with respect to all model components can be obtained and optimized simultaneously. While originally proposed to integrate scientific computing and machine learning (Innes et al. 2019, Rackauckas et al. 2020), differentiable programming can also be useful for flexible statistical modeling (Hackenberg et al. 2022a) and has been combined with statistical approaches, e.g., in an adaptation of neural ODEs for a Bayesian framework (Dandekar et al. 2021), or combinations of ODEs and non-linear mixed effects models for pharmacometric modeling (Rackauckas et al. 2022).

In our approach, we use the flexible automatic differentiation framework provided by Zygote.jl. (Innes et al. 2019) for jointly optimizing the dynamic model and the VAE for dimension reduction, such that the two components can influence each other. In this way, a latent representation can be found that is automatically adapted to the underlying dynamics and the ODE system structures and regularizes the representation. As the ODEs have analytical solutions, differentiation through the latent dynamics estimator does not require backpropagating gradients through a numerical ODE solving step. However, differentiable programming also allows for doing that efficiently if necessary, e.g., using the adjoint sensitivity method Chen et al. (2018).

The model is implemented in the Julia programming language (Bezanson et al. 2017) of version 1.7.2. with the additional packages CSV.jl (v0.10.9), DataFrames.jl (v1.2.2), Distributions.jl (v0.25.24), Flux.jl (v0.12.8) (Innes 2018), GLM.jl (v1.5.1), LaTeXStrings.jl (v1.3.0), MultivariateStats.jl (v0.8.0), Parameters.jl (v0.12.3), Plots.jl (v1.23.5) and StatsBase.jl (v0.33.21). The model is available as a Julia package at <https://github.com/mareha/LatentDynamics.jl>. The repository also provides Jupyter notebooks for illustrating usage of the approach and reproducing the results in the manuscript.

In the VAE, the encoder and decoder each have one hidden layer with the number of hidden units equal to the number of input dimensions and a tanh-activation functions. The latent space is two-dimensional, and the latent space mean and variance are obtained as affine linear transformations of the hidden layer values without a non-linear activation. Similarly, the decoder parameterizes mean and variance of a Gaussian distribution calculated from the decoder hidden layer using an affine linear transformation.

The network mapping baseline variables to ODE parameters has two hidden layers in addition to input and output layer. In the first hidden layer, the number of hidden units corresponds to the number of input variables and a tanh-activation is used. In the second hidden layer, the number of hidden units corresponds to the number of ODE parameters and the activation function is a sigmoid function, shifted by  $-0.5$  and scaled by  $0.5$  (resp.  $1$  in the simulation design). This effectively acts as a prior for the range of the estimated ODE parameters. Deviations from this range are possible, as an affine linear transformation

with a diagonal matrix is added as the final output layer.

In the loss function, the KL-divergence between the prior and posterior is scaled by a factor of 0.5 to slightly reduce the regularizing effect of the  $\mathcal{N}(0, 1)$  prior. The sum of the squared decoder parameters is added with a weighting factor of 0.01 to the loss function, corresponding to a commonly used penalty term to prevent exploding decoder parameters.

Additionally, the variance penalty term described in Section 3.2.2 of the main manuscript is added to the loss function with a weight of 2 in the SMartCARE example. This is not necessary for the simulation, as the variance is already controlled by the data generating process. The squared Euclidean distance between the posterior means from the encoded time series and from the individual ODE solutions for consistency of the latent representation before and after solving the ODEs is added with a weight of 1 in the SMartCARE application and a weight of 0.5 in the simulation. In the notation of Equation 6 in the main manuscript, we thus have  $\alpha = 1, \beta = 2$  for the SMartCARE example and  $\alpha = 0.5, \beta = 0$  in the simulation.

The models are trained based on stochastic gradient descent using the ADAM optimizer (Kingma & Ba 2015) with a learning rate of 0.0005 and 30 training epochs, chosen by monitoring convergence of the loss function and visualizing exemplary fits.

### 3 Sensitivity analysis

To empirically evaluate the robustness of our approach, we conducted a sensitivity analysis with different levels of noise, different numbers of individuals, and different numbers of time points per individual. Specifically, we vary  $\sigma_{\text{var}}^2 \in \{0.1, 0.5\}$ ,  $\sigma_{\text{ind}}^2 \in \{0.5, 1\}$ ,  $n \in \{50, 75, 100, 150, 250\}$  and  $T_{\text{max}} \in \{2, 5, 8, 15\}$ , where  $T_{\text{max}}$  denotes the maximum number of follow-up time points, from which we uniformly sample  $T_i$ , the number of observed time points for each individual. On each dataset, we fit the model and calculated the prediction error of the fitted trajectories in latent space. As a baseline performance reference, in each scenario and for each patient, we also computed a least squares regression fit of all previously observed encoded values at each observed time point, shifted the trajectory to start at the current observation and extrapolated until the next observation, as an adaptation of a regression-based approach to local predictions analogous to Figure 1 in the main manuscript. The results are shown in Figure 1.

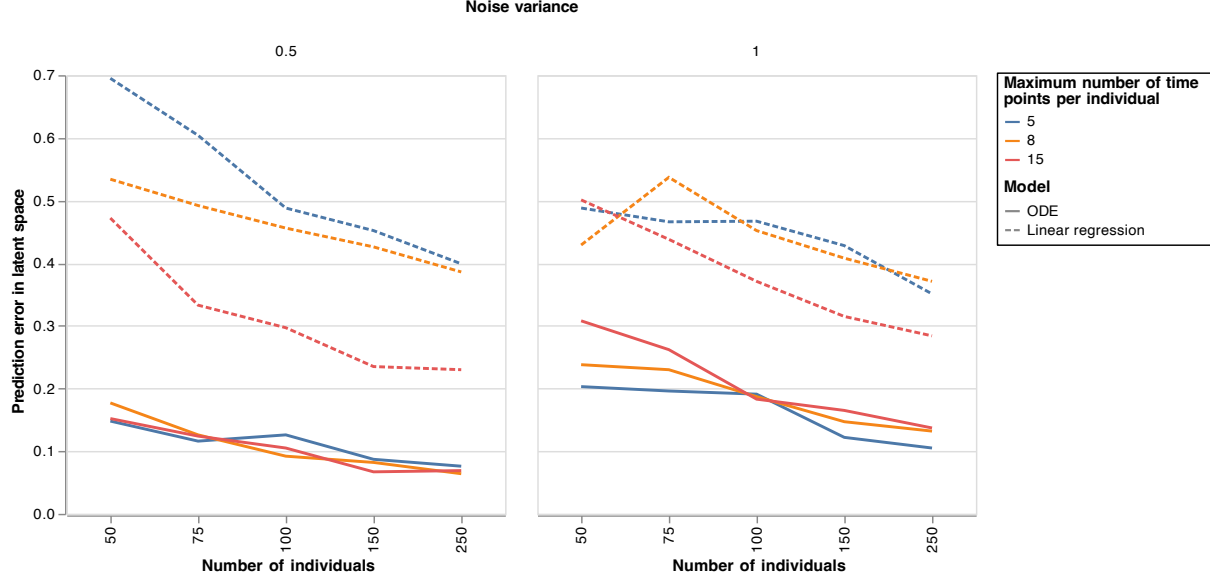

Figure 1: Results of a sensitivity analysis with different levels of noise in the data simulation and different numbers of individuals and time points per individual. On the  $y$ -axis, the mean squared prediction error in latent space across time points and patients is reported. The  $x$ -axis shows different numbers of simulated individuals. Solid lines correspond to the prediction errors of the ODE approach, while dashed lines correspond to the shifted regression approach as a performance reference. Different colors correspond to simulations with different numbers of time points per individual.

## 4 Simulation design with a simpler ODE system

In addition to the simulation using a homogeneous linear ODE with four unknown parameters from Section 4.1 in the main manuscript, we performed a simulation using a simpler two-dimensional system with just two unknown parameters. As before we defined two groups of individuals with distinct underlying development patterns. The corresponding ODE systems are given by

$$\begin{aligned} \frac{d}{dt} \begin{pmatrix} u_1 \\ u_2 \end{pmatrix} (t) &= \begin{pmatrix} -0.2 \\ 0.1 \end{pmatrix}; & \frac{d}{dt} \begin{pmatrix} u_1 \\ u_2 \end{pmatrix} (t) &= \begin{pmatrix} -0.1 \\ -0.2 \end{pmatrix}; \\ \begin{pmatrix} u_1 \\ u_2 \end{pmatrix} (0) &= \begin{pmatrix} 2 \\ 1 \end{pmatrix} & \begin{pmatrix} u_1 \\ u_2 \end{pmatrix} (0) &= \begin{pmatrix} 2 \\ 1 \end{pmatrix}. \end{aligned}$$

We simulated data for 100 individuals and trained our model on the data as described in 4.1 in the main manuscript. Exemplary fits from 12 simulated individuals are shown in Figure 2. Additionally, we show the fits of piecewise and global linear regression fits in Figures 3 and 3, as described in Section 4.1 in the main manuscript.

For the global regression model in Figure 4, we have calculated a regression fit using the complete observed time series of each patient, to empirically verify that our approach indeed matches a simple least-squared fit when underlying dynamics are simple.

For the piecewise regression model in Figure 3, we have calculated extrapolations based on previously observed values only, as discussed in Section 4.1 in the main manuscript. Naturally, this more limited observation leads to a drop in prediction performance, both when comparing predictions on subsequent time points in latent space and when decoding the respective predictions back to the level of the original items using the VAE decoder, as summarized below in Table 1.

| Model      | Prediction in latent space | Prediction on reconstructed values |
|------------|----------------------------|------------------------------------|
| ODE        | 0.406                      | 1.129                              |
| Regression | 0.981                      | 3.686                              |

Table 1: Mean squared error averaged across all time points and all simulated patients for predicting the subsequent time point both in latent space and on the level of the reconstructed items, using the ODE approach and a linear regression, fit on all previously observed data points.

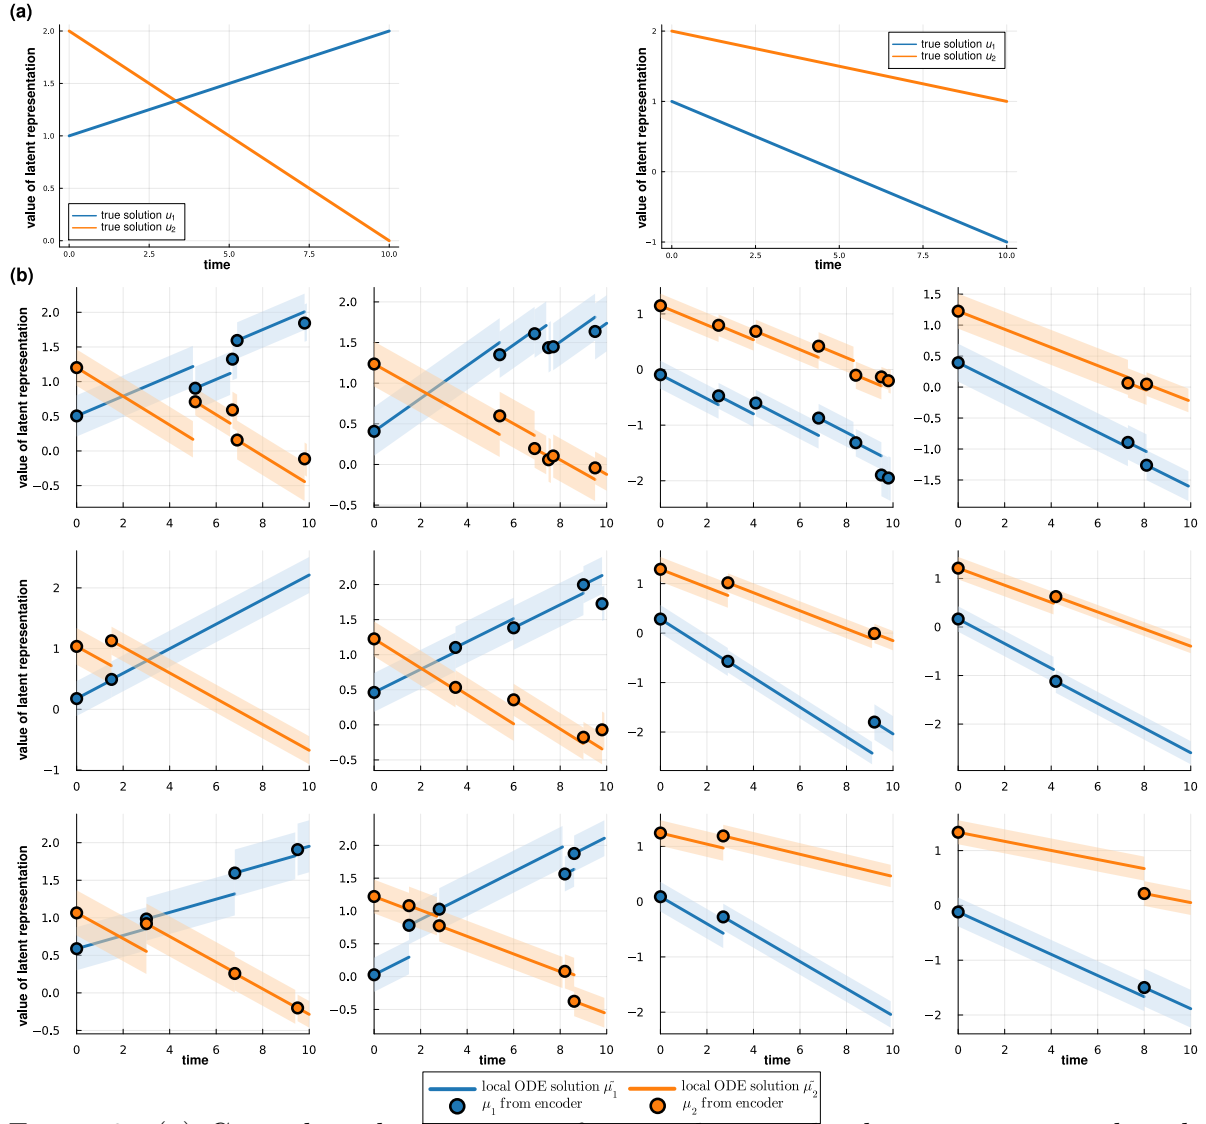

Figure 2: (a) Ground-truth trajectories for two distinct development patterns based on which data was simulated. (b) Exemplary fits of simulated individuals from both groups. One panel corresponds to one individual, the  $x$  axis shows the time and the  $y$  axis the value of the latent representation. Circles depict the mean of the latent variable as obtained directly from the encoder, while solid lines show the ODE solution with parameters obtained from the individual's baseline variables, using the value at the last observed time point as initial condition and solved until the subsequent time point. Colored bands show the range of one standard deviation of the latent variable around its mean. The two leftmost columns show 6 individuals from the first group corresponding to the left ground-truth trajectory in (a), while the two rightmost columns show 6 individuals from the second group, corresponding to the pattern shown on the right in (a).

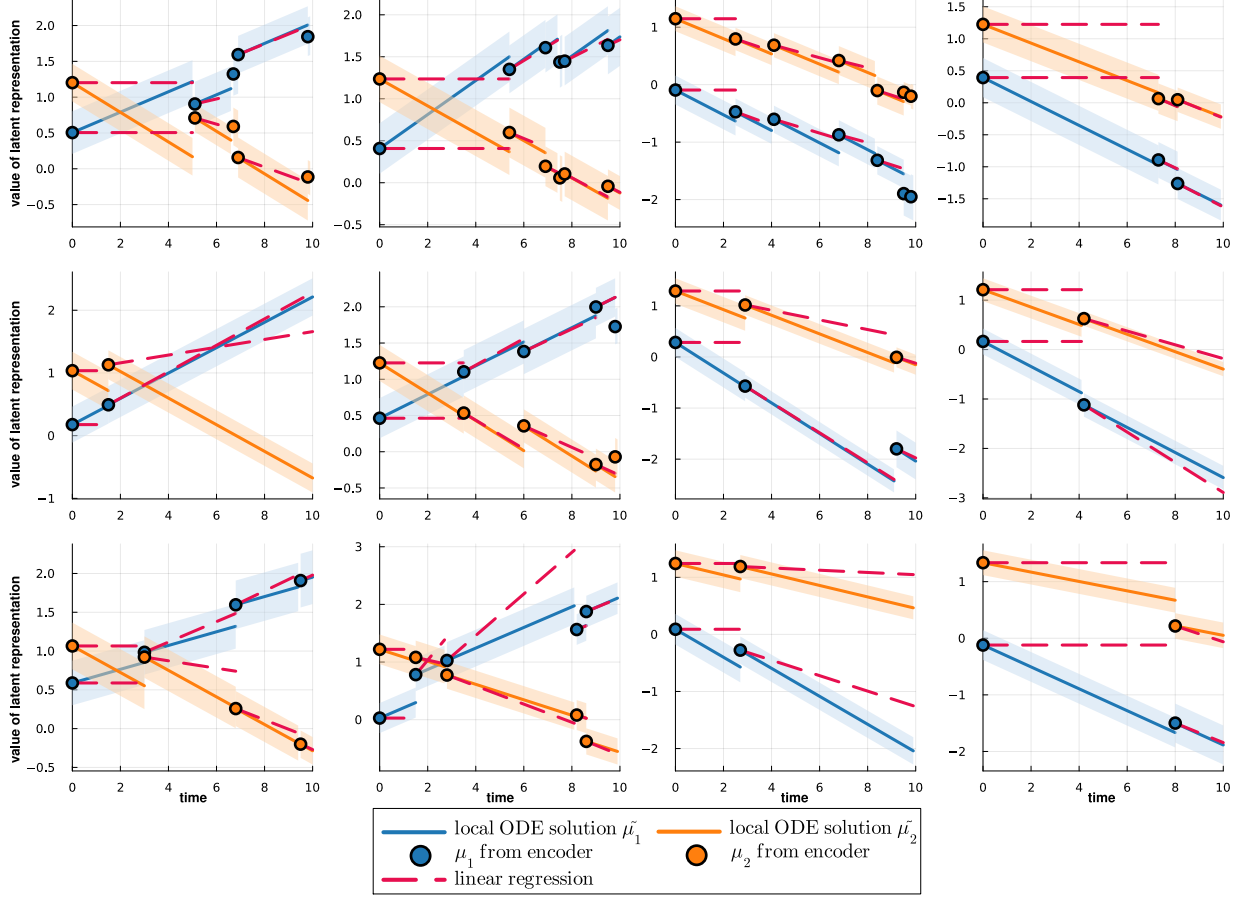

Figure 3: Exemplary fits of simulated individuals from Figure 2, with a piecewise linear regression fit shown in pink. For each simulated individual, at each time point in each latent dimension, a linear regression fit of all latent space values from previous time points of that individual and dimension was calculated. The regression line was shifted to the value of the last observation used for calculation, and extrapolated until the subsequent time point (corresponding to the adaptation of an initial value approach for a regression model discussed in Section 2 in the main text).

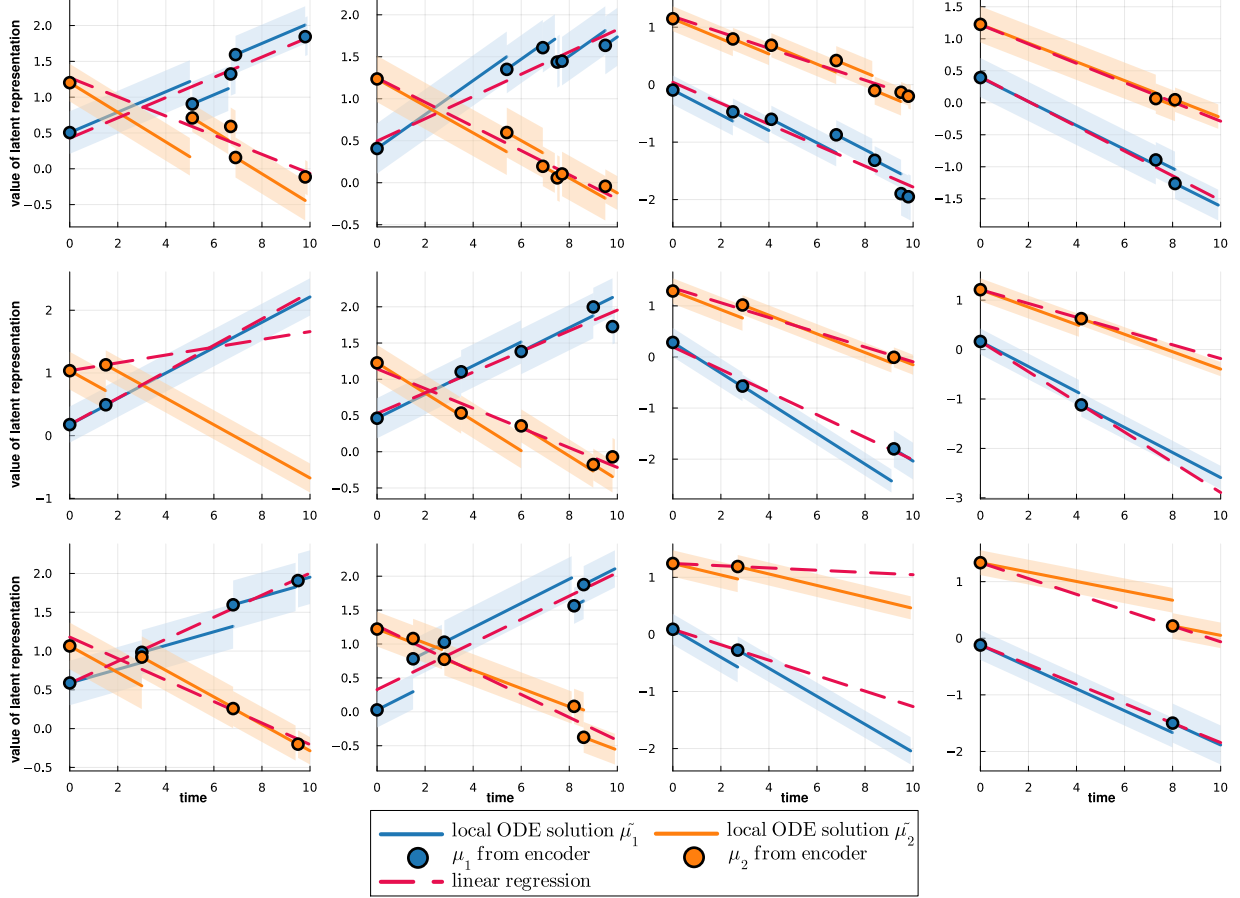

Figure 4: Exemplary fits of simulated individuals from Figure 2, with global linear regression fits shown in pink. For each simulated individual, in each latent dimension a linear regression fit of the complete time series of that individual and dimension was calculated (corresponding to the classical function fitting approach for regression models discussed in Section 2 in the main text).

## References

- Baydin, A. G., Pearlmutter, B. A., Radul, A. A. & Siskind, J. M. (2017), ‘Automatic differentiation in machine learning: A survey’, *J. Mach. Learn. Res.* **18**(1), 5595–5637.
- Bezanson, J., Edelman, A., Karpinski, S. & Shah, V. B. (2017), ‘Julia: A fresh approach to numerical computing’, *SIAM Review* **59**(1), 65–98.
- Chen, T. Q., Rubanova, Y., Bettencourt, J. & Duvenaud, D. (2018), Neural ordinary differential equations, *in* S. Bengio, H. M. Wallach, H. Larochelle, K. Grauman, N. Cesa-Bianchi & R. Garnett, eds, ‘Advances in Neural Information Processing Systems 31’, pp. 6572–6583.
- Dandekar, R., Chung, K., Dixit, V., Tarek, M., Garcia-Valadez, A., Vemula, K. V. &

- Rackauckas, C. (2021), ‘Bayesian neural ordinary differential equations’. arXiv preprint: <https://arxiv.org/abs/2012.07244>.
- Hackenberg, M., Grodd, M., Kreutz, C., Fischer, M., Esins, J., Grabenhenrich, L., Karagiannidis, C. & Binder, H. (2022a), ‘Using differentiable programming for flexible statistical modeling’, *The American Statistician* **76**(3), 270–279.
- Innes, M. (2018), ‘Flux: Elegant machine learning with Julia’, *Journal of Open Source Software* **3**(25), 602.
- Innes, M. (2019), ‘What is differentiable programming?’. Blogpost available at <https://fluxml.ai/blogposts/2019-02-07-what-is-differentiable-programming/> (date of retrieval: December 19, 2022).
- Innes, M., Edelman, A., Fischer, K., Rackauckas, C., Saba, E., Shah, V. B. & Tebbutt, W. (2019), ‘A differentiable programming system to bridge machine learning and scientific computing’. arXiv preprint: <https://arxiv.org/abs/1907.07587>.
- Kingma, D. P. & Ba, J. (2015), Adam: A method for stochastic optimization, *in* Y. Bengio & Y. LeCun, eds, ‘3rd International Conference on Learning Representations (ICLR), Conference Track Proceedings’.
- Rackauckas, C., Ma, Y., Martensen, J., Warner, C., Zubov, K., Supekar, R., Skinner, D. & Ramadhan, A. (2020), ‘Universal differential equations for scientific machine learning’. arXiv preprint: <https://arxiv.org/abs/2001.04385>.
- Rackauckas, C., Ma, Y., Noack, A., Dixit, V., Mogensen, P. K., Elrod, C., Tarek, M., Byrne, S., Maddhashiya, S., Calderón, J. S., Hatherly, M., Nyberg, J., Gobburu, J. V. S. & Ivaturi, V. (2022), ‘Accelerated predictive healthcare analytics with pumas, a high performance pharmaceutical modeling and simulation platform’, *bioRxiv* p. 2020.11.28.402297.
